# Supplementary material for: Learning from THEODORE: A Synthetic Omnidirectional Top-View Indoor Dataset for Deep Transfer Learning
Source: arXiv:2011.05719 source file (2020-11-11)
Supplement: Supplementary file 1 [file matrix.tex]

\setlength{\fboxsep}{0pt}
\begin{figure*}[ht!]
\captionsetup[subfigure]{labelformat=empty}
\centering
\begin{sideways}
    \hskip 0.13\textwidth
    \small \(FES\)
\end{sideways}
\begin{subfigure}[b]{0.4\textwidth}
    \caption{\(COCO\)}
    \fbox{\includegraphics[width=\textwidth]{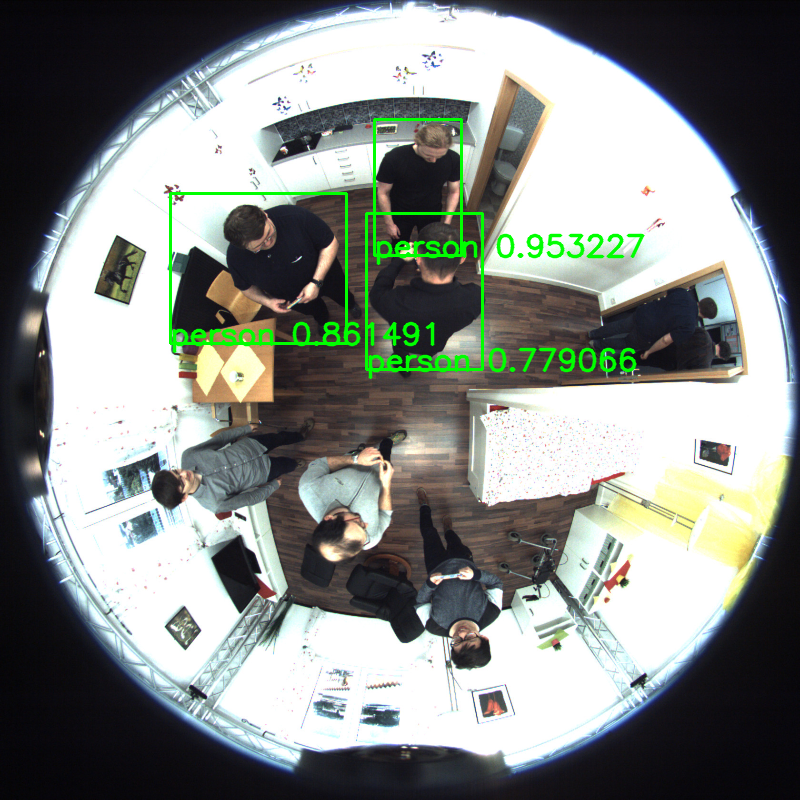}}
\end{subfigure}
\begin{subfigure}[b]{0.4\textwidth}
    \caption{\(THEODORE\)}
    \fbox{\includegraphics[width=\textwidth]{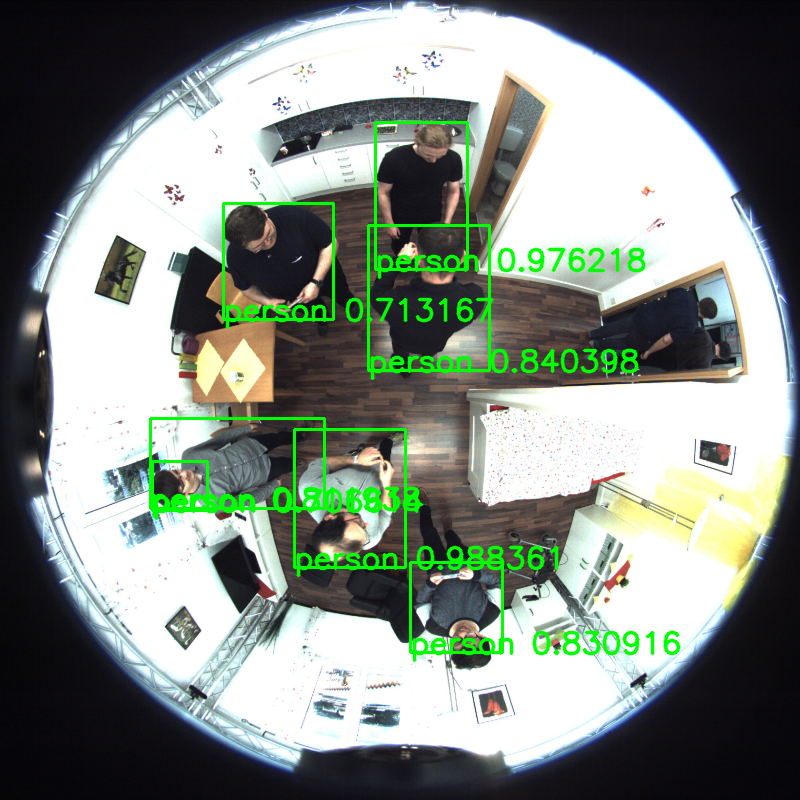}}
\end{subfigure}

\begin{sideways}
    \hskip 0.08\textwidth
    \small \(HDA\)
\end{sideways}
\begin{subfigure}[b]{0.4\textwidth}
    \fbox{\includegraphics[width=\textwidth]{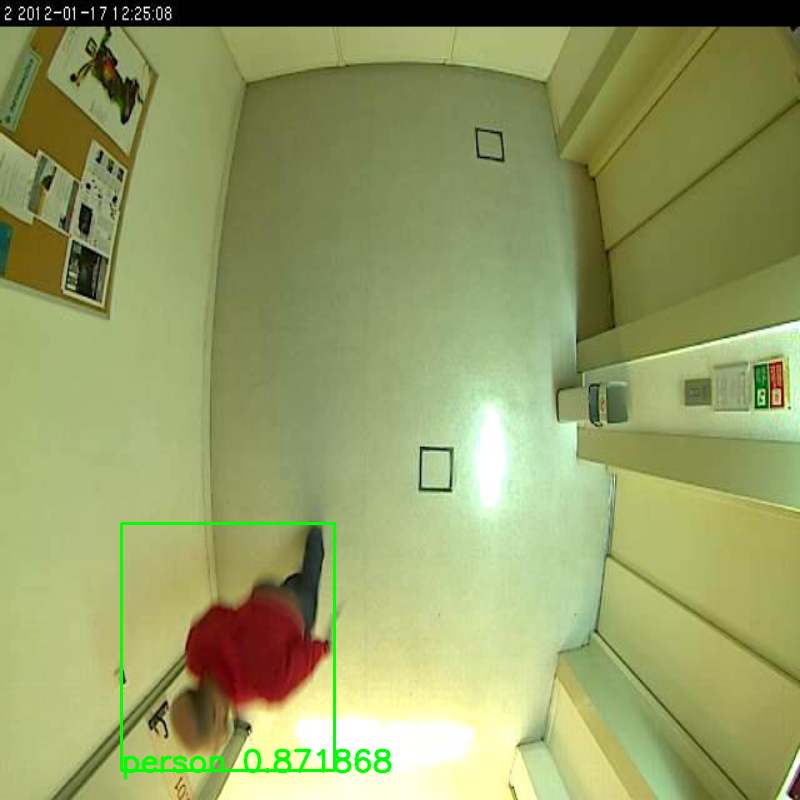}}
\end{subfigure}
\begin{subfigure}[b]{0.4\textwidth}
    \fbox{\includegraphics[width=\textwidth]{img/appendix/detection_results/faster_rcnn/theodore_frcnn_hda_00043.png}}
\end{subfigure}

\begin{sideways}
    \hskip 0.1\textwidth
    \small \(Bomni\)
\end{sideways}
\begin{subfigure}[b]{0.4\textwidth}
    \fbox{\includegraphics[width=\textwidth]{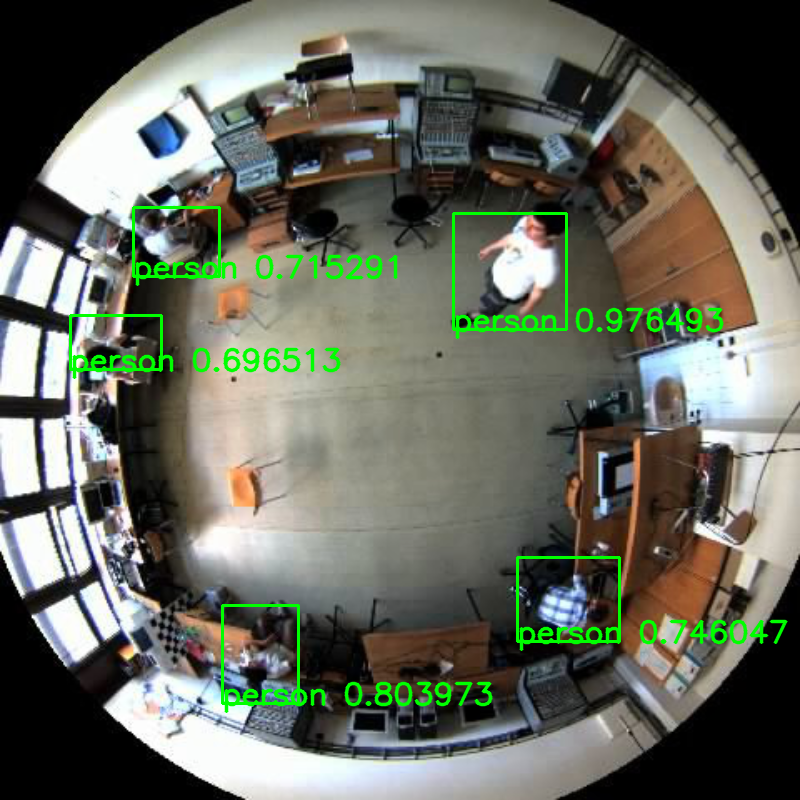}}
\end{subfigure}
\begin{subfigure}[b]{0.4\textwidth}
    \fbox{\includegraphics[width=\textwidth]{img/appendix/detection_results/faster_rcnn/theodore_frcnn_bomni_00025.png}}
\end{subfigure}
    \caption{Examples of Object detection results with Faster R-CNN \label{fig:appendix/detection_results_faster_rcnn/faster_rcnn}}
\end{figure*}
